# Supplementary material for: Glassy features of crystal plasticity
Source: arXiv:1607.07592 ancillary file (2016-07-26)
Supplement: Supplementary file 1 [file 3d_ddd_prb_SM.pdf]

# SUPPLEMENTAL MATERIAL: Glassy features of crystal plasticity

Arttu Lehtinen[1], Giulio Costantini[2], Mikko J. Alava[1], Stefano Zapperi[3,4,1], and Lasse Laurson[1]
[1] *COMP Centre of Excellence and Helsinki Institute of Physics, Department of Applied Physics, Aalto University, P.O.Box 11100, FI-00076 Aalto, Espoo, Finland.*
[2] *CNR-IENI, Via R. Cozzi 53, 20125 Milano, Italy*
[3] *ISI Foundation, Via Alassio 11/C, 10126 Torino, Italy and*
[4] *University of Milan, Via Celoria 16, 20133 Milano, Italy*

## VELOCITY-CONTROLLED VELOCITY AVALANCHES

### Complementary Cumulative Distributions

Complementary cumulative probability distribution functions (CDFs) are sometimes used instead of the probability densities [e.g. $P(s)$] to analyze the statistics of power law distributed quantities [1]. CDF of a quantity $x$ is given by $1 - C(x)$, where $C(x)$ is the cumulative distribution of $x$. The scaling exponent $\tau_{s,\mathrm{c}}$ of the power law section of the CDF of avalanche sizes $s$ is related to the scaling exponent $\tau_s$ of the corresponding probability density distribution via $\tau_{s,\mathrm{c}} = \tau_s - 1$; analogous relations hold for other quantities such as e.g. avalanche durations. In Figs. 1 and 2 we plot the CDFs corresponding to the probability densities $P_{\mathrm{INT}}(s)$ and $P(s)$ shown in the main article, respectively. From these, for both the integrated and stress-resolved cases, we obtain exponents that are in good agreement with the ones obtained from the corresponding probability densities: for large avalanches we have $\tau_{s,INT} = \tau_{s,\mathrm{INT,c}} + 1 = 1.54 \pm 0.0002$ and $\tau_s = \tau_{s,\mathrm{c}} + 1 = 1.32 \pm 0.0012$. From Fig. 2 one can also clearly see that the cutoff increases as a function of stress, highlighting again the fact that the avalanche dynamics is not stationary during the ramping up of the stress.

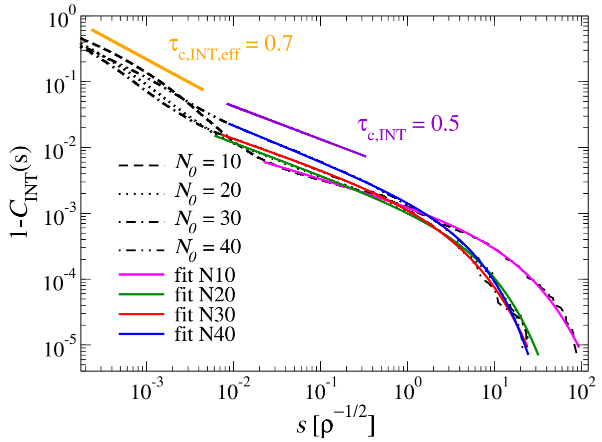


FIG. 1. Integrated complementary cumulative size distributions of the velocity avalanches, $1 - C_{\mathrm{INT}}(s)$, for different system sizes $N_0$. Above the small to large avalanche crossover, a power law scaling regime with $\tau_{s,\mathrm{INT,c}} = 0.5$ emerges.

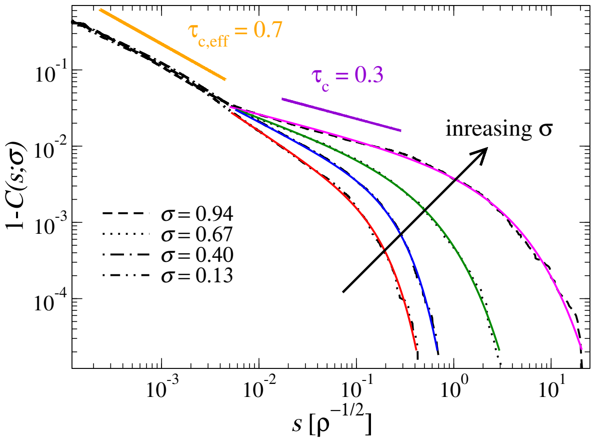


FIG. 2. Stress-resolved complementary cumulative size distributions of the velocity avalanches, $1 - C(s; \sigma)$, for the system size $N_0 = 40$. Above the small to large avalanche crossover, a power law scaling regime with $\tau_{s,\mathrm{c}} = 0.3$, terminated by a $\sigma$-dependent cut-off, emerges.

### Distributions of avalanche durations

For completeness, we present here also the distributions of the avalanche durations, as obtained by thresholding the velocity signal. Fig. 3 shows that the integrated distributions are characterized by $\tau_{T,\mathrm{INT}} = 1.5 \pm 0.17$. Fig. 4, showing the corresponding stress-resolved distributions, indicates that $\tau_T = 1.22 \pm 0.14$. Given this, and using the previously extracted $\tau_s = 1.15 \pm 0.13$, leads to an estimate of the exponent $\gamma$ via the scaling relation $\gamma = (\tau_T - 1)/(\tau_s - 1) = 1.47$, in excellent agreement with the result shown in the inset of Fig. 2 of the main article.

## STRAIN RATE CONTROLLED STRAIN AVALANCHES

In addition to the velocity controlled simulations, we also performed simulations where thresholding of the

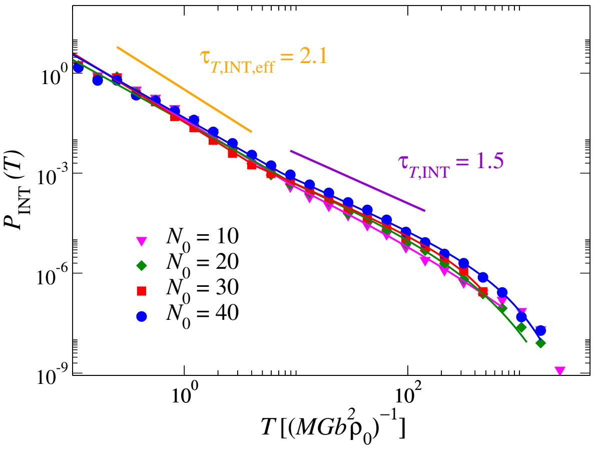


FIG. 3. Stress-integrated avalanche duration distributions $P_{\mathrm{INT}}(T)$ for different system sizes $N_0$. The large avalanche scaling region is characterized by an exponent $\tau_{T,\mathrm{INT}} = 1.5 \pm 0.1$.

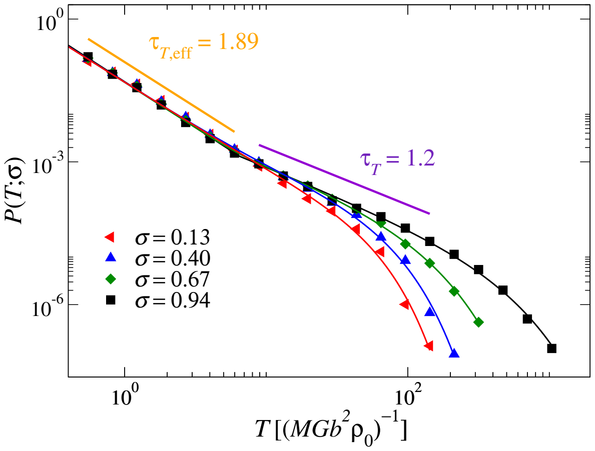


FIG. 4. Stress-resolved avalanche duration distributions $P(T)$ for different system sizes stress values for the system size $N_0 = 40$. The large avalanche scaling region is characterized by an exponent $\tau_T = 1.2 \pm 0.1$.

strain rate $\dot{\epsilon}$ was used to define the avalanches. The avalanche size $s'$ in these simulations was defined as the accumulated strain during an avalanche, corresponding to the length of the horizontal strain steps $\Delta\epsilon$ in the stress strain curves (see also Fig. 1 of the main article). The results of these simulations are presented in Figs. 5 and 6. As in the case of velocity avalanches, there are two different power law regimes. For small avalanches the scaling exponents are again given by $\tau_{s',INT,\mathrm{eff}} = 1.98 \pm 0.02$ and $\tau_{s',\mathrm{eff}} = 1.74 \pm 0.019$ for both distributions respectively. For larger avalanches we have $\tau_{s',\mathrm{INT}} = 1.48 \pm 0.03$ and $\tau_{s'} = 1.15 \pm 0.10$. For large avalanches the statistics are relatively poor, and hence the presence of a cut-off is not so clear as in the case of velocity avalanches or the velocity-controlled strain avalanches discussed above, and in the following Section.

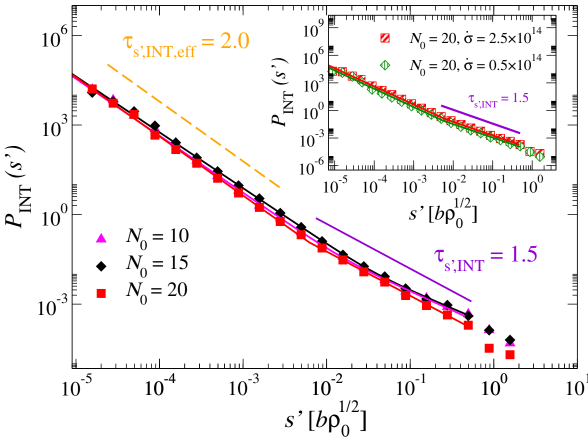


FIG. 5. Integrated strain avalanche distributions $P_{\mathrm{INT}}(s')$ of strainrate-controlled simulations for different system sizes $N_0$. Large enough avalanches are described by a power law with $\tau_{s',\mathrm{INT}} = 1.48 \pm 0.03$, while the smaller one are characterized by a larger effective $\tau_{s',\mathrm{INT,eff}} = 1.98 \pm 0.02$. The inset displays $P_{\mathrm{INT}}(s')$ of two sets of simulations with different rates of ramping up the stress between avalanches, showing that $P_{\mathrm{INT}}(s')$ does not depend on the stress rate.

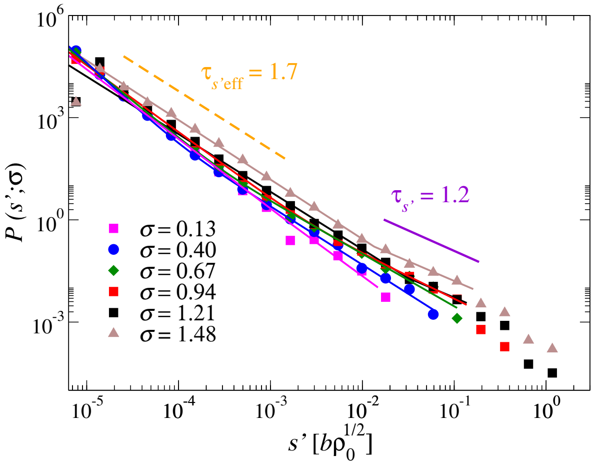


FIG. 6. Stress-resolved strain burst distributions $P(s';\sigma)$ of strainrate-controlled strain avalanches, with large enough avalanches described by a power-law with $\tau_{s'} = 1.15 \pm 0.10$. The data are for a system size $N_0 = 20$.

We checked also for the possibility of rate effects by changing the rate at which the stress is increased between avalanches. As can be seen from the inset of Fig. 5, varying the stress rate does not change the avalanche size distribution.

## VELOCITY CONTROLLED STRAIN AVALANCHES

Previous studies of simplified 2D discrete dislocation dynamics models have considered a protocol where the

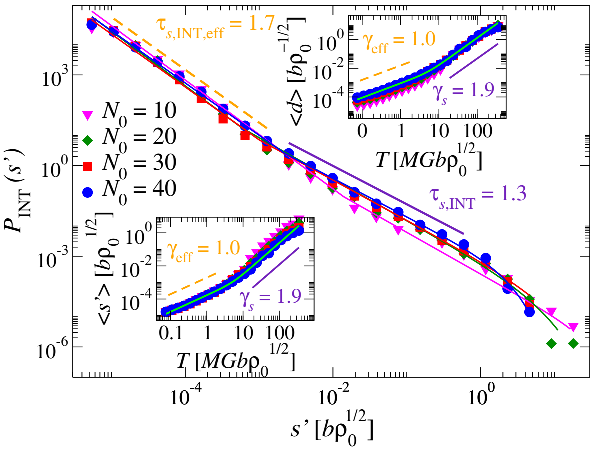


FIG. 7. Integrated size distributions $P(s')$ of velocity-controlled strain avalanches, with large enough avalanches described by a power-law with $\tau = 1.3 \pm 0.15$. The bottom left inset displays the average strain burst size $\langle s' \rangle$ as a function of burst duration $T$. The top right inset reveals that within the large avalanche scaling regime, the average slip $\langle d \rangle$ vs $T$ relation becomes independent of $N_0$.

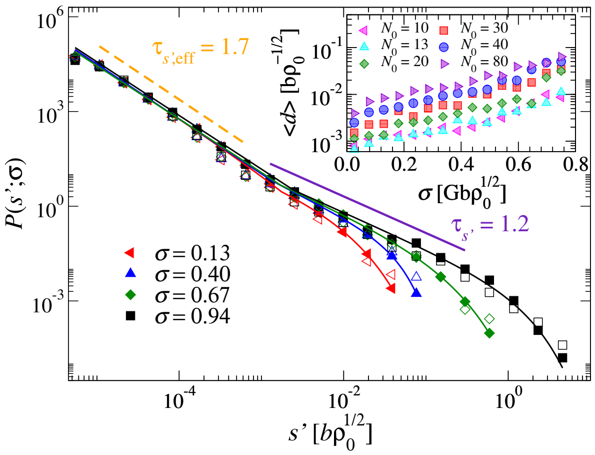


FIG. 8. The main panel shows stress resolved distributions $P(s';\sigma)$ of velocity-controlled strain avalanche sizes for the system sizes $N_0 = 40$ (filled symbols) and $N_0 = 30$ (empty symbols). Large enough avalanches are described by a power-law with $\tau = 1.159 \pm 0.18$. The (top right) inset shows the average amount of slip $d$ within the strain avalanches as a function of $\sigma$ for various $N_0$, revealing a growth of $\langle d \rangle$ with a dependence on both $\sigma$ and $N_0$.

collective velocity signal is used for thresholding to define the avalanches, but the avalanche size is still defined as the strain increment within such avalanches [2]. Thus, to be able to directly compare our results with such 2D simulations, ve consider such a protocol also in our 3D simulations; the results are shown in Figs. 7 and 8.

Both the integrated and stress-resolved avalanche size distributions exhibit similar $\tau$-exponents as in 2D simulations, i.e. $\tau_{s',\mathrm{INT}} = 1.3 \pm 0.15$ and $\tau_{s'} = 1.16 \pm 0.18$, respectively. This, together with the fact that also here the average slip avalanche size $\langle d \rangle = \langle s' \rangle L^2$ displays an exponential stress depedence with a prefactor diverging with the system size (insets of Fig. 8), indicates that both the simple 2D model(s) and the present, much more realistic and complex 3D system exhibit essentially the same, "glassy" avalanche dynamics. These values of the $\tau$-exponents are also essentially the same as those obtained using the other protocols to define avalanches discussed above.

In the bottom right inset of Fig. 7, we show also the average size $\langle s'(T) \rangle$ of the avalanches as a function of the avalanche duration $T$. A power law emerges in the region of large $T$, but the curves corresponding to different system sizes have a slightly different amplitude in the scaling regime. This is similar to the results obtained for velocity avalanches (main article). However, the exponent is different ($\gamma = 1.91$ vs $\gamma = 1.5$). In the top right inset of Fig. 7 we have plotted the average slip $\langle d \rangle = \langle s' \rangle L^2$ as function of $T$. By considering $d$ instead of $s$, a collapse of the $\langle d(T) \rangle$ curves is obtained (i.e. their amplitude becomes independent of $N_0$) in the power law scaling region.

## EFFECT OF CROSS-SLIP

Our main results were simulated with the dislocations constrained to their glide-planes as no cross-slip was allowed for the segments with screw character. To check the robustness of our results we did one batch of simulations with the cross-slip activated. The stress resolved velocity avalanche size distribution follows a power-law with similar exponent $\tau_s = 1.21 \pm 0.18$ for large avalanches as was the case without cross-slip as can be seen in the main panel of Fig. 9. The bottom left inset shows that the stress integrated avalanche size distribution follows a power-law for large avalanches with $\tau_{s,INT,eff} = 1.47 \pm 0.08$ which is consistent with our main results. The total dislocation activity $\langle s \rangle D_{\mathrm{tot}}$ shows exponential $\sigma$ dependence $\langle s \rangle D_{\mathrm{tot}} \sim A\exp(\sigma/\sigma_0)$ but for even wider range of stresses when compared to the no cross-slip case.

## EFFECT OF DIFFERENT INITIAL STATES

In order to study the effect of the different initial states to the avalanche dynamics, we did a batch of simulations where initial dislocation configurations were taken from simulations of the main section that were at stress $\sigma = 1.1$ and then relaxed before quasistatic loading was started again. The stress resolved avalanche size distributions of these simulations are of the similar functional form as the ones in obtained in the main section of the paper. Large avalanches follow a power-law with a size exponent $\tau_s = 1.11 \pm 0.24$ which is very close to the

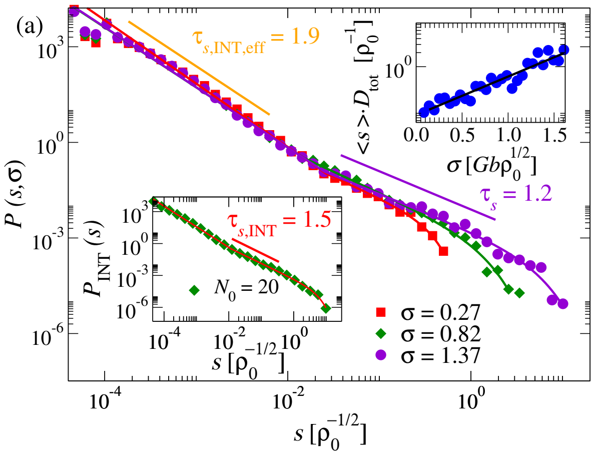


FIG. 9. The main panel shows stress resolved distributions $P(s';\sigma)$ of velocity-controlled velocity avalanche sizes when cross-slip is activated for the system size $N_0 = 20$. Large enough avalanches are described by a power-law with $\tau_s = 1.2 \pm 0.1$. The bottom left inset shows the stress integrated avalanche distribution where large enough avalanches are described by a power-law with $\tau_{s,INT} = 1.47 \pm 0.08$ The top right inset shows the average amount of dislocation activity $\langle s \rangle D_{\mathrm{tot}}$ within the avalanches as a function of $\sigma$, revealing a roughly exponential $\sigma$ dependence $\langle s \rangle D_{\mathrm{tot}} \sim A\exp(\sigma/\sigma_0)$. (bottom left inset).

value obtained earlier. The cut-off of the distribution increases when stress increases which again consistent with the main results. These features can be seen in the main panel of Fig. 10. The average stress-strain curve of the stressed simulations differs from the original one by being more steep at small stresses and strains. This corresponds to the fact the dislocation avalanches are smaller in the beginning of the loading when the stress is small. This trend is evident from the top right inset of Fig. 10 where the aver-age avalanche size as function of stress is plotted for both the original and stressed systems. Possible explanation to this difference is that for the stressed case, the big avalanches which are triggered by small stresses, have already happened and thus the systems starts from a deeper valley in the potential landscape. When stress is increased to the value $\sigma = 1.1$, the average avalanche size is approximately the same for both cases i.e the stressed system has forgotten its initial state.

[1] R. Maaß, M. Wraith, J. T. Uhl, J. R. Greer, and K. A. Dahmen, Slip statistics of dislocation avalanches under different loading modes, Phys. Rev. E **91**, 042403 (2015).

[2] P. D. Ispánovity, L. Laurson, M. Zaiser, I. Groma, S. Zapperi, and M. J. Alava, Avalanches in 2D Dislocation Systems: Plastic Yielding Is Not Depinning, Phys. Rev. Lett. **112**, 235501 (2014).

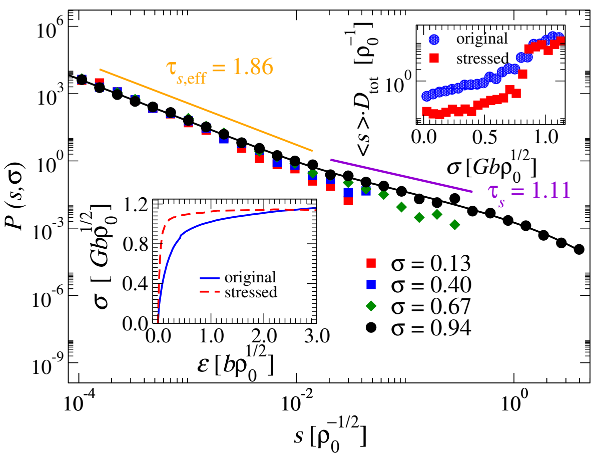


FIG. 10. The main panel shows stress resolved distributions $P(s';\sigma)$ of velocity-controlled velocity avalanche sizes when stressed initial configurations are used. System size is $N_0 = 40$. Large enough avalanches are described by a power-law with $\tau_s = 1.11 \pm 0.24$. The top right inset shows the average amount of dislocation activity $\langle s \rangle D_{\rm tot}$ within the avalanches as a function of $\sigma$. For stresses $\sigma_0 \lesssim 1.0$ the mean avalanche size is smaller for the pre-stressed initial configurations. The bottom left inset shows the average stress strain curves obtained by using both the stressed and the non-stressed initial configurations.
